# Supplementary material for: Rethinking Class-Incremental Learning from a Dynamic Imbalanced Learning Perspective
Source: arXiv:2405.15157 source file (2024-05-24)
Supplement: Supplementary file 1 [file supp_ablation.tex]

\begin{figure}[!h]
\centering 
\begin{tikzpicture} %tikz图片

\begin{axis}[
    xlabel=Number of seen classes, 
    ylabel=Top-1 Accuracy, 
    tick align=outside, 
    legend pos=north east
    ]

\addplot[smooth,mark=*,red] plot coordinates {
(10,91.10)
(20,60.50)
(30,49.70)
(40,42.40)
(50,40.30)
(60,38.80)
(70,37.30)
(80,31.52)
(90,29.52)
(100,27.14)
};
\addlegendentry{baseline}

\addplot[smooth,mark=+,blue] plot coordinates {
(10,90.90)
(20,66.75)
(30,55.70)
(40,46.72)
(50,45.00)
(60,42.42)
(70,41.80)
(80,39.80)
(90,38.57)
(100,37.16)
};
\addlegendentry{baseline+fm}

\addplot[smooth,mark=x,green] plot coordinates {
(10,91.00)
(20,67.60)
(30,57.30)
(40,47.45)
(50,44.12)
(60,40.95)
(70,39.07)
(80,38.31)
(90,36.62)
(100,35.41)
};
\addlegendentry{baseline+dm}

\addplot[smooth,mark=star,yellow] plot coordinates {
(10,91.70)
(20,72.20)
(30,69.20)
(40,61.22)
(50,57.34)
(60,52.03)
(70,50.73)
(80,45.35)
(90,42.37)
(100,40.62)
};
\addlegendentry{up}

\addplot[smooth,mark=diamond,orange] plot coordinates {
(10,90.10)
(20,69.80)
(30,71.87)
(40,67.32)
(50,63.72)
(60,62.02)
(70,60.00)
(80,56.30)
(90,53.93)
(100,51.78)
};
\addlegendentry{up+dm}

\addplot[smooth,mark=triangle,cyan] plot coordinates {
(10,91.70)
(20,73.05)
(30,71.33)
(40,65.25)
(50,62.20)
(60,60.07)
(70,57.60)
(80,54.90)
(90,53.00)
(100,51.12)
};
\addlegendentry{up+fm}

\end{axis}
\end{tikzpicture}
\caption{Top-1 accuracy curves in ablation study}
\label{fig:supp_ablation}
\end{figure}
